# Supplementary material for: From local spin nematicity to altermagnets: Footprints of band topology
Source: arXiv:2403.14620 ancillary file (2025-05-02)
Supplement: Supplementary file 1 [file Supplementary_AltMag_1.pdf]

# Supplemental Material: From Local Spin Nematicity to Altermagnets: Footprints of Band Topology

Sanjib Kumar Das[1] and Bitan Roy[1]

[1]*Department of Physics, Lehigh University, Bethlehem, Pennsylvania, 18015, USA*

(Dated: April 8, 2024)

This Supplemental Material contains (a) energetics of spin nematic orders and the phase locking therein in monolayer graphene (MLG), Bernal bilayer graphene (BBLG) and rhombohedral trilayer graphene (RTLG) [Sec. S1 and Fig. S1], and (b) topology of altermagnets with trigonal warping in BBLG and RTLG [Sec. S2 and Fig. S2].

## S1. ENERGETICS OF SPIN NEMATIC ORDERS IN MLG, BBLG AND RTLG

In this section, we discuss the energetics of the spin nematic orders in MLG, BBLG and RTLG. In the latter two systems, we now incorporate the trigonal warping terms. For simplicity, we neglect the Nambu doubling, and consider only the sublattice/layer, valley and spin degrees of freedom. We also omit the Zeeman coupling. Then the low-energy free fermion Hamiltonian in these systems respectively takes the form

$$\begin{aligned}
\hat{h}_{\rm MLG}(\boldsymbol{k}) &= \alpha_1 \left[\Gamma_{031} k_x - \Gamma_{002} k_y\right], \\
\hat{h}_{\rm BBLG}(\boldsymbol{k}) &= \alpha_2 \left[\Gamma_{001} \left(k_x^2 - k_y^2\right) + \Gamma_{032} \left(2 k_x k_y\right)\right] + \alpha_1 \left[\Gamma_{031} k_x - \Gamma_{002} k_y\right], \\
\hat{h}_{\rm RTLG}(\boldsymbol{k}) &= \alpha_3 \left[\Gamma_{031} \left\{k_x \left(k_y^2 - 3k_x^2\right)\right\} + \Gamma_{002} \left\{k_y \left(3k_x^2 - k_y^2\right)\right\}\right] + \alpha_0 \Gamma_{001}. \qquad \text{(S1)}
\end{aligned}$$

Eight-component Hermitian $\Gamma$ matrices take the form $\Gamma_{\nu\rho\lambda} = \sigma_\nu \tau_\rho \beta_\lambda$, where $\{\sigma_\kappa\}$, $\{\tau_\kappa\}$, $\{\beta_\kappa\}$ are two-component Pauli matrices for $\kappa = 0, \cdots, 3$, operating on the spin, valley and sublattice or layer indices, respectively. In BBLG, the term proportional to $\alpha_1$, and in RTLG, the term proportional to $\alpha_0$ capture the trigonal warping.

The spin nematic orders in all these systems, transforming under the $E_g$ and $E_u$ representations of $D_{3d}$ group are captured by the following effective single-particle Hamiltonian [see also Eq. (2) of the main manuscript]

$$\hat{h}^{\rm spin}_{E_g}\left(\Delta_{E_g}, \theta_{E_g}\right) = \Delta_{E_g}\left[\Gamma_{301}\cos\theta_{E_g} + \Gamma_{332}\sin\theta_{E_g}\right] \ \text{and}\ \hat{h}^{\rm spin}_{E_u}\left(\Delta_{E_u}, \theta_{E_u}\right) = \Delta_{E_u}\left[\Gamma_{331}\cos\theta_{E_u} + \Gamma_{302}\sin\theta_{E_u}\right], \quad \text{(S2)}$$

respectively. For simplicity, we have taken $\theta_j \to -\theta_j$ for $j = E_g$ and $E_u$. The condensation energy gain in the presence of spin nematic orders is

$$\Delta E(\Delta_j, \theta_j) = \sum_{\alpha \in filled} \int \frac{d^2\boldsymbol{k}}{(2\pi)^2} \Big[E_\alpha(\Delta_j, \theta_j, \boldsymbol{k}) - E_\alpha(0, 0, \boldsymbol{k})\Big], \quad \text{(S3)}$$

where $E_\alpha(\Delta_j, \theta_j, \boldsymbol{k})$ $[E_\alpha(0, 0, \boldsymbol{k})]$ are the eigenvalues of the total effective single-particle Hamiltonian with (without) the spin nematic order [see also Eq. (3) of the main manuscript] are given by

$$\hat{h}^{\rm alt}_j(\Delta_j, \theta_j) = \hat{h}_{\rm a}(\boldsymbol{k}) + \hat{h}^{\rm spin}_j(\Delta_j, \theta_j), \quad \text{(S4)}$$

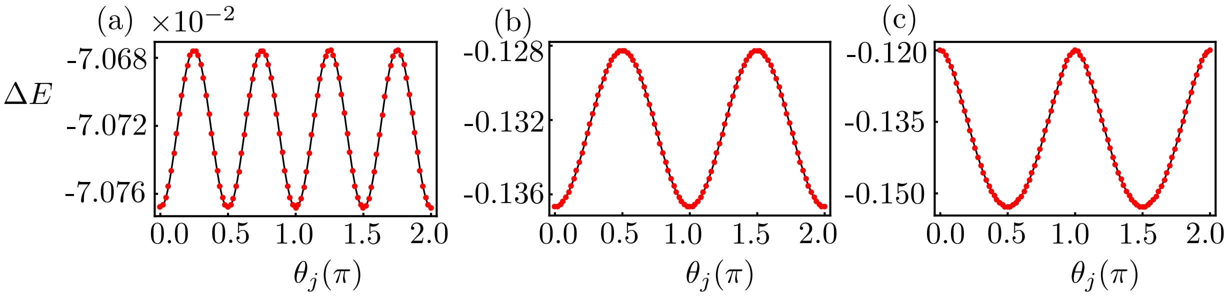


Figure S1. Condensation energy gain in the spin nematic ordered phases [see Eq. (S3)], as a function of $\theta_j$ in (a) MLG, (b) BBLG and (c) RTLG. The results are identical for $j = E_g$ and $E_u$ spin nematic orders. The results are obtained for (a) $\alpha_1 = 1.0$ and $\Delta_j = 0.2$, (b) $\alpha_2 = 1.0$, $\alpha_1 = 0.15$ and $\Delta_j = 0.2$, and (c) $\alpha_3 = 1.0$, $\alpha_0 = 0.15$ and $\Delta = 0.2$ [Eqs. (S1) and (S2)].

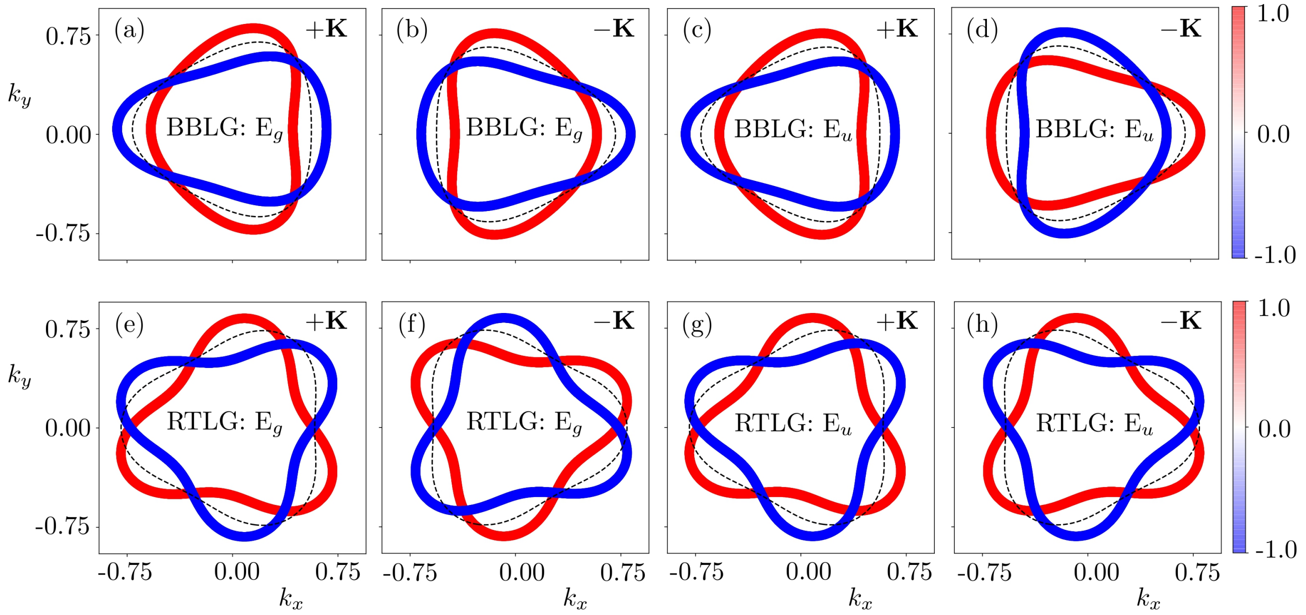


Figure S2. Constant energy ($E = 0.40$ for BBLG and $E = 0.35$ for RTLG) contours for spin up (red) and down (blue) fermions near the inequivalent valleys at $+\mathbf{K}$ [(a), (c), (e) and (g)] and $-\mathbf{K}$ [(b), (d), (f) and (h)] in BBLG [(a)-(d)] and RTLG [(e)-(h)] in the $E_g$ [(a), (b), (e) and (f)] and $E_u$ [(c), (d), (g) and (h)] spin nematic phases with trigonal warping therein. The results are obtained for $\theta_j = 0$ in BBLG and $\theta_j = \pi/2$ in RTLG for $j = E_g$ and $E_u$ [see Eq. (S2)]. They correspond to the minimal energy configurations [Fig. S1]. Other parameter values are the following: $\alpha_2 = 1.0$, $\alpha_1 = 0.15$ and $\Delta_j = 0.2$ [(a)-(d)] and $\alpha_3 = 1.0$, $\alpha_0 = 0.15$ and $\Delta = 0.2$ [(e)-(h)]. See Eqs. (S1) and (S2). Black dashed lines represent spin degenerate three-fold symmetric Fermi surfaces of free fermions ($\Delta_j = 0$) for the same parameter values. The numbers in the color bar represent the spin projection in the $z$-direction (in units of $\hbar/2$). In BBLG (RTLG) $\alpha_1$ ($\alpha_0$) captures trigonal warping [Eq. (S1)].

where a = MLG, BBLG and RTLG. Summation (indexed by $\alpha$) in Eq. (S3) is performed over all the filled states at negative energies, and the integral over momentum ($\boldsymbol{k}$) is replaced by a summation over a large but finite number of points in the reciprocal space. We ensure that the quantity $\Delta E(\Delta_j, \theta_j)$ has converged with respect to the number of points in the reciprocal space. The results are shown in Fig. S1. It turns out that $\Delta E(\Delta_j, \theta_j)$ is identical for $j = E_g$ and $E_u$, but shows nontrivial dependence on $\theta_j$, indicating the underlying nematicity in the ordered state. This outcome clearly reflects from the fact that $\Delta E(\Delta_j, 0) \neq \Delta E(\Delta_j, \pi/2)$. We find that in MLG and BBLG the minimal energy configuration corresponds to $\theta_j = 0$, while that in RTLG corresponds to $\theta_j = \pi/2$.

## S2. TOPOLOGY OF ALTERMAGNETS WITH TRIGONAL WARPING IN BBLG AND RTLG

In this section, we discuss the topology of constant energy contours for opposite spin projections in two spin nematic phases in BBLG and RTLG after accounting for the trigonal warping therein. The results are shown in Fig. S2. The constant energy contours for free fermions are no longer rotationally symmetric, rather displays discrete three-fold ($C_3$) symmetry. Such contours for opposite spin projections also enclose equal area in the reciprocal space, which we confirm explicitly within the numerical accuracy, hence yielding altermagnet with no net magnetic moment. Furthermore and most importantly, the constant energy contours for spin-up and spin-down electrons whenever cross each other, always intersect *four* and *six* times in BBLG and RTLG, respectively. Therefore, they always represent $d$-wave and $f$-wave altermagnets, respectively, which we announced in the main manuscript without the trigonal warping terms. In MLG, there is no trigonal warping term up to energy $\sim$ 1eV. The effect of Zeeman coupling of in-plane magnetic fields is the same as shown in the right column of Fig. 1 of the main manuscript. It gaps out the crossing points between the constant energy contours of opposite spin projections. Thus, we do not show them explicitly here.
